# Supplementary material for: SPIGAN: Privileged Adversarial Learning from Simulation
Source: arXiv:1810.03756 source file (2019-02-18)
Supplement: Supplementary file 1 [file supplementary_material.tex]

%\onecolumn

\section*{Supplementary Material}
\label{sec:supmat}

\setlength{\parindent}{1pc}

Our supplementary materials includes: a video (spigan.avi, use VLC media player to view) showing how the outputs of the task network $T$ and privileged network $P$ change during training, (ii) additional details about our hyper-parameters in Section~\ref{sec:supmathparams}, (iii) our early stopping criterion in Section~\ref{sec:supmatearlystop}, and (iv) additional qualitative image generation results in Figure~\ref{fig:supp_qualitative_cityscapes} (Cityscapes experiments) and Figure~\ref{fig:supp_qualitative_vistas} (Vistas experiments).

%%%%%%%%%%%%%%%%%%%%%%
% TODO: Kuan & Adrien
\subsection{Hyper-parameters}
\label{sec:supmathparams}

In this section we give additional details about the hyper-parameters used in our experiments.

All the networks are trained from scratch (except the ImageNet-pretrained VGG19 network used for the perceptual loss).
We use the Adam optimizer with $\beta_1=0.5$. We use a learning rate fixed to 0.0002 for the first 100 epochs, and then linearly decayed to zero over the next 100 epochs.

When loading images, we resize them by fixing a width of 256 pixels and keep the original aspect ratio.

For data augmentation, we randomly flip 50\% of the images, and randomly crop a fixed region (128 $\times$ 256).

In general, we use the following configurations for all the experiments:
\begin{itemize}
\setlength\itemsep{0mm}
\item{batch size of 32;}
\item{Gaussian initialization with zero mean and 0.02 standard deviation;}
\item{dropout with probability of 50\% after every ReLU layer of each residual block in the generator;}
\item{Leaky ReLU activations with a leakiness of 0.2.}
\end{itemize}

\paragraph{CycleGAN}
\begin{itemize}
\setlength\itemsep{0mm}
\item{We use instance normalization for normalization layers in both $G$ and $D$.}
\item{We set $\lambda=10$ for controlling the importance of cycle consistency.}
\end{itemize}

\paragraph{PixelDA}
\begin{itemize}
\setlength\itemsep{0mm}
\item{Input noise vector with $N^z=100$ is sampled from $\mathcal{U}(-1,1)$.}
\item{We set the importance of adversarial loss $\alpha=1$, task-specific loss $\beta=0.5$, content-similarity loss (as well as perceptual loss in our application) $\gamma=0.33$.}
\item{We use batch normalization for normalization layers in both $G$ and $D$.}
\end{itemize}

\paragraph{SPIGAN}
\begin{itemize}
\setlength\itemsep{0mm}
\item{We use inverse depth extracted from the z-buffer as privileged information: it avoids setting an arbitrary clipping distance and handles sky pixels more robustly.} % TODO more details? eq?
\item{We use batch normalization for normalization layers in both $G$ and $D$.}
\end{itemize}

\subsection{Early Stopping}
\label{sec:supmatearlystop}

%Setting hyper-parameters in unsupervised settings without a validation set is an open challenge.
%%
%Although it is possible to use prior knowledge or standard hyper-parameters for learning rates, finding the right number of iterations is important for adversarial learning methods.
%
As our main goal is to improve generalization performance in the target domain and we do not have validation sets, we use early stopping based on the training losses to avoid overfitting to the simulation domain.

Figure~\ref{fig:training_loss} shows the GAN losses of the different networks.
The task loss is not shown for clarity, as it always converges.
We select the stopping epoch roughly when the GAN loss converges (e.g., SPIGAN on Vistas) or when the discriminator and generator losses diverge.
Note that in the more frequent latter case, the discriminator always dominates the generator. 
% , see Table~\ref{tab:epoch_selection}.

For the SYNTHIA-to-Cityscapes experiments where all methods partially address the domain gap, we select 100 epochs for all methods.
For the SYNTHIA-to-Vistas experiments, we use 60 epochs for CycleGAN, 50 for PixelDA, 150 for SPIGAN.

We experimentally validated that aggressive early stopping for CycleGAN and PixelDA is necessary on Vistas due to negative transfer (i.e. results get worse after).
In contrast, we find that on Vistas the PI regularization in SPIGAN means it is slower to learn as it is more conservative (as seen in the qualitative results in Figure~\ref{fig:supp_qualitative_vistas}).

\clearpage

%\begin{supptable}[h]
%\centering
%\vspace{-2mm}
%\begin{tabular}{l|c|c|}
%\cline{2-3}
%                               & \multicolumn{1}{l|}{SYNTHIA $\rightarrow$ Cityscapes} & \multicolumn{1}{l|}{SYNTHIA $\rightarrow$ Vistas} \\ \hline
%\multicolumn{1}{|l|}{CycleGAN} & 100                                       & 60                                    \\ \hline
%\multicolumn{1}{|l|}{PixelDA}  & 100                                       & 50                                    \\ \hline
%\multicolumn{1}{|l|}{SPIGAN}   & 100                                       & 150                                   \\ \hline
%\end{tabular}
%\vspace{-2mm}
%\caption{Number of epochs selected with our early stopping criterion.}
%\label{tab:epoch_selection}
%\end{supptable}

\begin{suppfigure*}
\centering
\begin{subfigure}[t]{0.49\textwidth}
    \includegraphics[width=\textwidth]{figures/supplements/early_stopping/smoothy/cycle_gan_cityscapes.png}
    \includegraphics[width=\textwidth]{figures/supplements/early_stopping/smoothy/pixel_da_cityscapes.png}
    \includegraphics[width=\textwidth]{figures/supplements/early_stopping/smoothy/spi_gan_cityscapes.png}
    %\caption{SYNTHIA $\rightarrow$ Cityscapes}
\end{subfigure}
\begin{subfigure}[t]{0.49\textwidth}
    \includegraphics[width=\textwidth]{figures/supplements/early_stopping/smoothy/cycle_gan_vistas.png}
    \includegraphics[width=\textwidth]{figures/supplements/early_stopping/smoothy/pixel_da_vistas.png}
    \includegraphics[width=\textwidth]{figures/supplements/early_stopping/smoothy/spi_gan_vistas.png}
    %\caption{SYNTHIA $\rightarrow$ Vistas}
\end{subfigure}
\vspace{-2mm}
\caption{Training GAN losses of each approach (loss\_D for discriminators and loss\_G for generators). Left column is for SYNTHIA $\rightarrow$ Cityscapes adaptation, and right column is for SYNTHIA $\rightarrow$ Vistas adaptation.}
\label{fig:training_loss}
%\vspace{-35mm}
\end{suppfigure*}

\newpage

%%%%%%%%%%%%%%%%%%%%%%
% TODO: Jie & Kuan
%\subsection{Additional Generated Images}
%\label{sec:supmatres}

\begin{suppfigure*}
\centering
\vspace*{-10mm}
\begin{subfigure}[t]{0.24\textwidth}
    \includegraphics[width=\textwidth]{figures/supplements/cityscaeps/synthia/SYNTHIA-SEQS-02-DAWN_000182.png}
    \includegraphics[width=\textwidth]{figures/supplements/cityscaeps/synthia/SYNTHIA-SEQS-02-DAWN_000057.png}
    \includegraphics[width=\textwidth]{figures/supplements/cityscaeps/synthia/SYNTHIA-SEQS-04-FALL_000650.png}
    \includegraphics[width=\textwidth]{figures/supplements/cityscaeps/synthia/SYNTHIA-SEQS-02-DAWN_000095.png}
    \includegraphics[width=\textwidth]{figures/supplements/cityscaeps/synthia/SYNTHIA-SEQS-04-FALL_000349.png}
    \includegraphics[width=\textwidth]{figures/supplements/cityscaeps/synthia/SYNTHIA-SEQS-04-FALL_000398.png}
    \includegraphics[width=\textwidth]{figures/supplements/cityscaeps/synthia/SYNTHIA-SEQS-04-FALL_000632.png}
    \includegraphics[width=\textwidth]{figures/supplements/cityscaeps/synthia/SYNTHIA-SEQS-04-FALL_000636.png}
    \caption{Synthetic images}
\end{subfigure}
\begin{subfigure}[t]{0.24\textwidth}
    \includegraphics[width=\textwidth]{figures/supplements/cityscaeps/cycle_gan/SYNTHIA-SEQS-02-DAWN_000182.png}
    \includegraphics[width=\textwidth]{figures/supplements/cityscaeps/cycle_gan/SYNTHIA-SEQS-02-DAWN_000057.png}
    \includegraphics[width=\textwidth]{figures/supplements/cityscaeps/cycle_gan/SYNTHIA-SEQS-04-FALL_000650.png}
    \includegraphics[width=\textwidth]{figures/supplements/cityscaeps/cycle_gan/SYNTHIA-SEQS-02-DAWN_000095.png}
    \includegraphics[width=\textwidth]{figures/supplements/cityscaeps/cycle_gan/SYNTHIA-SEQS-04-FALL_000349.png}
    \includegraphics[width=\textwidth]{figures/supplements/cityscaeps/cycle_gan/SYNTHIA-SEQS-04-FALL_000398.png}
    \includegraphics[width=\textwidth]{figures/supplements/cityscaeps/cycle_gan/SYNTHIA-SEQS-04-FALL_000632.png}
    \includegraphics[width=\textwidth]{figures/supplements/cityscaeps/cycle_gan/SYNTHIA-SEQS-04-FALL_000636.png}
    \caption{CycleGAN}
\end{subfigure}
\begin{subfigure}[t]{0.24\textwidth}
    \includegraphics[width=\textwidth]{figures/supplements/cityscaeps/pixel_da/SYNTHIA-SEQS-02-DAWN_000182.png}
    \includegraphics[width=\textwidth]{figures/supplements/cityscaeps/pixel_da/SYNTHIA-SEQS-02-DAWN_000057.png}
    \includegraphics[width=\textwidth]{figures/supplements/cityscaeps/pixel_da/SYNTHIA-SEQS-04-FALL_000650.png}
    \includegraphics[width=\textwidth]{figures/supplements/cityscaeps/pixel_da/SYNTHIA-SEQS-02-DAWN_000095.png}
    \includegraphics[width=\textwidth]{figures/supplements/cityscaeps/pixel_da/SYNTHIA-SEQS-04-FALL_000349.png}
    \includegraphics[width=\textwidth]{figures/supplements/cityscaeps/pixel_da/SYNTHIA-SEQS-04-FALL_000398.png}
    \includegraphics[width=\textwidth]{figures/supplements/cityscaeps/pixel_da/SYNTHIA-SEQS-04-FALL_000632.png}
    \includegraphics[width=\textwidth]{figures/supplements/cityscaeps/pixel_da/SYNTHIA-SEQS-04-FALL_000636.png}
    \caption{PixelDA*}
\end{subfigure}
\begin{subfigure}[t]{0.24\textwidth}
    \includegraphics[width=\textwidth]{figures/supplements/cityscaeps/spigan/SYNTHIA-SEQS-02-DAWN_000182.png}
    \includegraphics[width=\textwidth]{figures/supplements/cityscaeps/spigan/SYNTHIA-SEQS-02-DAWN_000057.png}
    \includegraphics[width=\textwidth]{figures/supplements/cityscaeps/spigan/SYNTHIA-SEQS-04-FALL_000650.png}
    \includegraphics[width=\textwidth]{figures/supplements/cityscaeps/spigan/SYNTHIA-SEQS-02-DAWN_000095.png}
    \includegraphics[width=\textwidth]{figures/supplements/cityscaeps/spigan/SYNTHIA-SEQS-04-FALL_000349.png}
    \includegraphics[width=\textwidth]{figures/supplements/cityscaeps/spigan/SYNTHIA-SEQS-04-FALL_000398.png}
    \includegraphics[width=\textwidth]{figures/supplements/cityscaeps/spigan/SYNTHIA-SEQS-04-FALL_000632.png}
    \includegraphics[width=\textwidth]{figures/supplements/cityscaeps/spigan/SYNTHIA-SEQS-04-FALL_000636.png}
    \caption{SPIGAN}
\end{subfigure}
\vspace{-2mm}
%\caption{Qualitative results of adaptation from SYNTHIA to Cityscapes.}
\caption{Qualitative results of adaptation from SYNTHIA to Cityscapes.}
\label{fig:supp_qualitative_cityscapes}
\vspace{-25mm}
\end{suppfigure*}

\begin{suppfigure*}
\centering
\begin{subfigure}[t]{0.24\textwidth}
    \includegraphics[width=\textwidth]{figures/supplements/vistas/synthia/SYNTHIA-SEQS-01-DAWN_000132.png}
    \includegraphics[width=\textwidth]{figures/supplements/vistas/synthia/SYNTHIA-SEQS-01-DAWN_000509.png}
    \includegraphics[width=\textwidth]{figures/supplements/vistas/synthia/SYNTHIA-SEQS-01-DAWN_001050.png}
    \includegraphics[width=\textwidth]{figures/supplements/vistas/synthia/SYNTHIA-SEQS-01-DAWN_001111.png}
    \includegraphics[width=\textwidth]{figures/supplements/vistas/synthia/SYNTHIA-SEQS-02-FALL_000002.png}
    \includegraphics[width=\textwidth]{figures/supplements/vistas/synthia/SYNTHIA-SEQS-02-SPRING_000802.png}
    \includegraphics[width=\textwidth]{figures/supplements/vistas/synthia/SYNTHIA-SEQS-04-SUMMER_000288.png}
    \includegraphics[width=\textwidth]{figures/supplements/vistas/synthia/SYNTHIA-SEQS-06-SPRING_000674.png}
    \caption{Synthetic images}
\end{subfigure}
\begin{subfigure}[t]{0.24\textwidth}
    \includegraphics[width=\textwidth]{figures/supplements/vistas/cycle_gan/SYNTHIA-SEQS-01-DAWN_000132.png}
    \includegraphics[width=\textwidth]{figures/supplements/vistas/cycle_gan/SYNTHIA-SEQS-01-DAWN_000509.png}
    \includegraphics[width=\textwidth]{figures/supplements/vistas/cycle_gan/SYNTHIA-SEQS-01-DAWN_001050.png}
    \includegraphics[width=\textwidth]{figures/supplements/vistas/cycle_gan/SYNTHIA-SEQS-01-DAWN_001111.png}
    \includegraphics[width=\textwidth]{figures/supplements/vistas/cycle_gan/SYNTHIA-SEQS-02-FALL_000002.png}
    \includegraphics[width=\textwidth]{figures/supplements/vistas/cycle_gan/SYNTHIA-SEQS-02-SPRING_000802.png}
    \includegraphics[width=\textwidth]{figures/supplements/vistas/cycle_gan/SYNTHIA-SEQS-04-SUMMER_000288.png}
    \includegraphics[width=\textwidth]{figures/supplements/vistas/cycle_gan/SYNTHIA-SEQS-06-SPRING_000674.png}
    \caption{CycleGAN}
\end{subfigure}
\begin{subfigure}[t]{0.24\textwidth}
    \includegraphics[width=\textwidth]{figures/supplements/vistas/pixel_da/SYNTHIA-SEQS-01-DAWN_000132.png}
    \includegraphics[width=\textwidth]{figures/supplements/vistas/pixel_da/SYNTHIA-SEQS-01-DAWN_000509.png}
    \includegraphics[width=\textwidth]{figures/supplements/vistas/pixel_da/SYNTHIA-SEQS-01-DAWN_001050.png}
    \includegraphics[width=\textwidth]{figures/supplements/vistas/pixel_da/SYNTHIA-SEQS-01-DAWN_001111.png}
    \includegraphics[width=\textwidth]{figures/supplements/vistas/pixel_da/SYNTHIA-SEQS-02-FALL_000002.png}
    \includegraphics[width=\textwidth]{figures/supplements/vistas/pixel_da/SYNTHIA-SEQS-02-SPRING_000802.png}
    \includegraphics[width=\textwidth]{figures/supplements/vistas/pixel_da/SYNTHIA-SEQS-04-SUMMER_000288.png}
    \includegraphics[width=\textwidth]{figures/supplements/vistas/pixel_da/SYNTHIA-SEQS-06-SPRING_000674.png}
    \caption{PixelDA*}
\end{subfigure}
\begin{subfigure}[t]{0.24\textwidth}
    \includegraphics[width=\textwidth]{figures/supplements/vistas/spigan/SYNTHIA-SEQS-01-DAWN_000132.png}
    \includegraphics[width=\textwidth]{figures/supplements/vistas/spigan/SYNTHIA-SEQS-01-DAWN_000509.png}
    \includegraphics[width=\textwidth]{figures/supplements/vistas/spigan/SYNTHIA-SEQS-01-DAWN_001050.png}
    \includegraphics[width=\textwidth]{figures/supplements/vistas/spigan/SYNTHIA-SEQS-01-DAWN_001111.png}
    \includegraphics[width=\textwidth]{figures/supplements/vistas/spigan/SYNTHIA-SEQS-02-FALL_000002.png}
    \includegraphics[width=\textwidth]{figures/supplements/vistas/spigan/SYNTHIA-SEQS-02-SPRING_000802.png}
    \includegraphics[width=\textwidth]{figures/supplements/vistas/spigan/SYNTHIA-SEQS-04-SUMMER_000288.png}
    \includegraphics[width=\textwidth]{figures/supplements/vistas/spigan/SYNTHIA-SEQS-06-SPRING_000674.png}
    \caption{SPIGAN}
\end{subfigure}
\vspace{-2mm}
\caption{Qualitative results of adaptation from SYNTHIA to Vistas.}
\label{fig:supp_qualitative_vistas}
% \vspace{-20mm}
\end{suppfigure*}
